# Supplementary material for: Recovering a Clipped Signal in Sparseland
Source: arXiv:1110.5063 source file (2011-10-23)

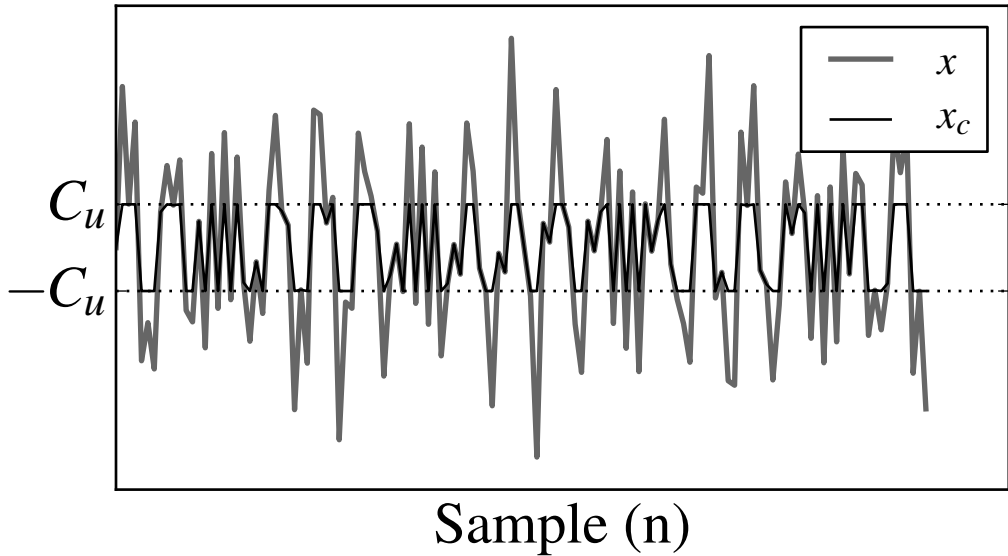

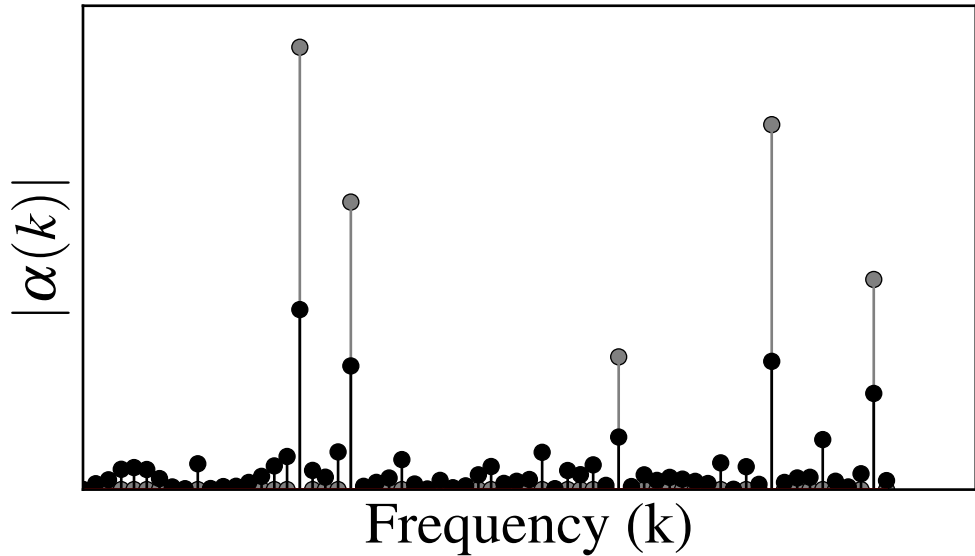

Supplement: Supplementary file 1 [file supp_estimation.pdf]
